# Supplementary material for: LLM-Powered Analysis of IoT User Reviews: Tracking and Ranking Security and Privacy Concerns
Source: arXiv:2601.00372 source file (2026-01-01)
Supplement: Supplementary file 1 [file Appendix.tex]

\newpage
\section{List of Products from The Wild Dataset $\mathcal{W}$}\label{products}
\subsection{Fitness Tracker: 23 ASINS, 24046 reviews}
% Please add the following required packages to your document preamble:
% \usepackage{booktabs}
\begin{table}[h]
\centering
\resizebox{0.5\textwidth}{!}{\begin{tabular}{@{}llr@{}}
\toprule
\textbf{ASIN} & \textbf{Product}                  & \multicolumn{1}{l}{\textbf{No. of Reviews}} \\ \midrule
B09BXQ4HMB    & Fitbit Charge 5                   & 4783                                        \\
B08DFGPTSK    & Fitbit Inspire 2                  & 4760                                        \\
B08DKYLK4D    & Amazfit Band 5                    & 4670                                        \\
B08XM8X4VQ    & KALINCO Smart Watch               & 3118                                        \\
B09LMD1WL4    & Kummel Fitness Tracker            & 1075                                        \\
B08PF9V27X    & ENGERWALL Fitness Tracker         & 896                                         \\
B0B5FGP237    & Fitbit Inspire 3                  & 809                                         \\
B09PRHRTKG    & Pautios Smart Watch               & 802                                         \\
B0BCWQ6P99    & KAKTIN Smart Watch                & 609                                         \\
B0BVLVBYPJ    & Smart Watch Fitness Tracker       & 470                                         \\
B09M3LQ6WB    & threesheep Fitness Tracker        & 444                                         \\
B09QBVD7BY    & aeac Smart Watch                  & 411                                         \\
B0BLYV4B1L    & DoSmarter Fitness Tracker         & 297                                         \\
B0C1N9VDMM    & Ddidbi Smart Watch                & 199                                         \\
B0BTBX691N    & Fitness Tracker(Answer/Make Call) & 175                                         \\
B0BY89CPDQ    & ASWEE Smart Watch                 & 169                                         \\
B0BW43XJ94    & TOOBUR Smart Watch                & 141                                         \\
B0BR9TBF8Q    & WalkerFit A1 Smart Watch          & 130                                         \\
B0BTPHY136    & Fitness Tracker                   & 44                                          \\
B0BTZ4SN9S    & Fitness Tracker                   & 24                                          \\
B0C3XWPM18    & Fitness Tracker                   & 18                                          \\
B09BXH5MC1    & Fitbit Charge 5                   & 1                                           \\
B0BVLWKNKR    & Smart Watch Fitness Tracker       & 1                                           \\ \bottomrule
\end{tabular}}
\end{table}
\subsection{Smart Speaker: 24 ASINS, 32179 reviews}
% Please add the following required packages to your document preamble:
% \usepackage{booktabs}
\begin{table}[H]
\centering
\resizebox{0.5\textwidth}{!}{
\begin{tabular}{@{}llr@{}}
\toprule
\textbf{ASIN}       & \textbf{Product}                        & \multicolumn{1}{l}{\textbf{No. of Reviews}} \\ \midrule
B06XXM5BPP & Echo (2nd Gen)                 & 4911                               \\
B07G9Y3ZMC & Echo Studio                    & 4516                               \\
B07XKF5RM3 & Echo (4th Gen)                 & 4354                               \\
B07XJ8C8F5 & Echo Dot (4th Gen)             & 4323                               \\
B07FZ8S74R & Echo Dot (3rd Gen)             & 4140                               \\
B07F2H1LHL & XLeader SoundAngel A8          & 2424                               \\
B09B8W5FW7 & Echo Dot (5th Gen)             & 1495                               \\
B07NJPXRBC & Sonos One (Gen 2)              & 1038                               \\
B07W6RYRZM & Sonos One SL                   & 880                                \\
B07FDF9B46 & Bose Home Speaker 500          & 873                                \\
B08MQYNHWD & Sonos Move                     & 814                                \\
B08VKXP1VY & Bose SoundLink Revolve II      & 591                                \\
B09QC4X5S4 & SEREONIC TV Speakers           & 419                                \\
B084KYM1HH & Refurbished Echo Dot (4th Gen) & 373                                \\
B07NQD5L6V & Refurbished Echo Studio        & 362                                \\
B085PNV4SK & Refurbished Echo (4th Gen)     & 229                                \\
B08HPXPTSB & Belkin SOUNDFORM Elite         & 145                                \\
B07PN63DCP & Sonos One (Gen 2)              & 75                                 \\
B077GK3TTQ & Sonos Two Room Set             & 68                                 \\
B09SJ4RL8M & Precision Pro Ace GPS Speaker  & 52                                 \\
B09Q82T1ZL & BESTISAN 100W Subwoofer        & 38                                 \\
B09R4ZF2QW & Turtlebox Gen 2                & 27                                 \\
B09R4XLCV3 & Turtlebox Gen 2                & 18                                 \\
B09R4YXC7W & Turtlebox Gen 2                & 14                                 \\ \bottomrule
\end{tabular}}
\end{table}
%\newpage
\subsection{Security Camera: 28 ASINS, 35524 reviews}
% Please add the following required packages to your document preamble:
% \usepackage{booktabs}
\begin{table}[H]
\centering
\resizebox{.5\textwidth}{!}{
\begin{tabular}{@{}llr@{}}
\toprule
\textbf{ASIN} & \textbf{Product}                  & \multicolumn{1}{l}{\textbf{No. of Reviews}} \\ \midrule
B086DKMSSM    & Blink Outdoor (3rd Gen)           & 4719                                        \\
B07X6C9RMF    & Blink Mini Indoor Camera          & 4537                                        \\
B0758L64L9    & Ring Spotlight Cam                & 4097                                        \\
B08B3B3LQ3    & Arlo Spotlight Camera             & 3905                                        \\
B0B5GRGB58    & Wireless Outdoor Cameras          & 3385                                        \\
B08GHX9G5L    & Kasa Pan/Tilt Camera              & 2762                                        \\
B07X5FCW3X    & Blink Indoor (3rd Gen)            & 2036                                        \\
B0BD5VXKGW    & Galayou 2K Indoor Camera          & 1512                                        \\
B0866S3D82    & TP-Link Tapo Indoor Camera        & 1424                                        \\
B0BJ6XQ78R    & Wireless Cameras                  & 1341                                        \\
B00L3W2QJ2    & ANNKE 3K Camera System            & 724                                         \\
B09HC4ZJBL    & LaView 4MP Cameras                & 719                                         \\
B0BKG4Z1NK    & IHOXTX Cameras                    & 691                                         \\
B016UCNP3A    & REOLINK 5MP Camera System         & 605                                         \\
B09P33NVRF    & 2K (3MP) Cameras                  & 504                                         \\
B09Q38Y8NH    & Acelerar 2K Outdoor Camera        & 474                                         \\
B00NBT224O    & ZOSI 1080p Camera System          & 430                                         \\
B09J6Y8Y73    & Nest Indoor Cam                   & 304                                         \\
B0BJBH3XGZ    & Tashi Light Bulb Camera           & 284                                         \\
B08WFJKK2T    & Arlo Indoor Camera                & 253                                         \\
B082KGF6FX    & REOLINK 4K Camera System          & 231                                         \\
B0B5VLCL1N    & Blink Floodlight Camera           & 215                                         \\
B0BX9ZKQKT    & Outdoor Wireless Cameras          & 148                                         \\
B0816DWCD5    & Hiseeu 5MP Wired Camera System    & 122                                         \\
B0BX3MJHN6    & Gerdviaw 2K Cameras               & 88                                          \\
B0BMKK2SX5    & Camland Solar Camera System       & 10                                          \\
B086DKSHQ4    & Blink Outdoor (3rd Gen)           & 2                                           \\
B08PBR83NM    & Blink Mini Indoor Camera (3-Pack) & 2                                           \\ \bottomrule
\end{tabular}}
\end{table}

\newpage
\input{Section/apdx_crc}
\newpage
\input{Section/apdx_tm}
% \newpage
% \input{Section/apdx_camera_quotes}
